# Supplementary material for: Looking Beyond Sentence-Level Natural Language Inference for Downstream Tasks
Source: arXiv:2009.09099 source file (2020-09-18)
Supplement: Supplementary file 1 [file extra_info_appendix.tex]

%%%%%%%%%%%%%%%% Gain/Loss analysis on RACE subset %%%%%%%%%%%%%%%%%%%%%
Figures \ref{fig:gain_dist} and \ref{fig:loss_dist} show the distribution of labels over the Gain and Loss regions respectively. The distribution reflects that the

\hspace{-15mm}
\includegraphics[width=0.6\textwidth]{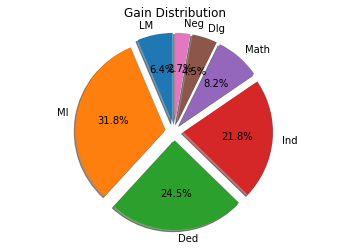}
\caption{Distribution of Reasoning Categories over the Gain region - Rule-based NLI vs QA model}
\label{fig:gain_dist}
\end{figure}

\begin{figure}[h]
    \hspace{-15mm}
    \includegraphics[width=0.6\textwidth]{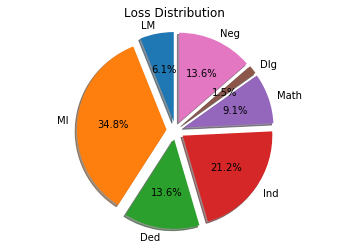}
    \caption{Distribution of Reasoning Categories over the Loss region - Rule-based NLI vs QA model.}
    \label{fig:loss_dist}
\end{figure}

%%%%%%%%%%%%%%%%%%%%%%%%%%%%%%%%%%%%%%%%%%%%%%%%%%%%%%%%%%%%%%%%%%%%%%%%%

%%%%%%%%%%%%%%%%%%%%%%%%%%%% RACE heuristic categories %%%%%%%%%%%%%%%%%%%
As a consequence of the rule-based conversion strategy, we unintentionally get 2 very different sets of data from the RACE dataset. $83\%$ of the RACE-subset consists of questions with question-words such as \{\textit{who, what, when, where, why, which, how}\} whereas only $1\%$ of the rest of the RACE dataset has such questions. Conversely, only about $11\%$ of the subset consists of fill-in-the-blanks (FITB) questions whereas $95\%$ of the rest of the dataset has FITB questions. {FITB questions are largely with the blank towards the end of the question and a question-answer concatenation strategy turns out to be very similar to a coherent conversion strategy. We argue that this is the reason for equivalent performance of the models on the FITB part of the data. However, on the RACE-subset, NLI models are able to outperform the QA model which showing the clear benefits of coherent conversion on complex question formulations.}

In order to compare the models trained using the neural and hybrid conversion to the rule-based conversion, we define some non-exclusive categories using heuristics, as described in Table \ref{tab:heuristic_categories}. We observe that the NLI model which uses the hybrid conversion gets a significantly better performance on the deductive reasoning category than the NLI model which uses the rule-based conversion. This observation is consistent with the trend seen in the comparison of the rule-based model vs the QA model, where the rule-based model outperforms the QA model on the deductive reasoning category. Additionally, the rule-based model outperforms the QA model significantly in the dialogue category. Table \ref{tab:heuristic_categories_perf} shows the performance of the models on the RACE-subset dataset over these question types. This trend further emphasizes the benefits of proper hypothesis generation as opposed to question and answer concatenation for the question-answering task.

\begin{table}[]
    \centering
    \begin{tabular}{c|c|c|c}
        \toprule
        \textbf{Type} & \textbf{QA} & \textbf{Rule-based} & \textbf{Hybrid}\\
        \bottomrule
        Main Idea & 84.19 & \textbf{84.83} & \textbf{84.83}\\\hline
        Negation & \textbf{80.86} & 77.77 & 79.01\\\hline
        Dialogue & 80.65 & \textbf{83.60} & 82.95\\\hline
        Math & 45 & \textbf{55} & \textbf{55}\\\hline
        Deductive & 81.91 & 88.29 & \textbf{90.42}\\\hline
        FITB & 79.02 & 79.02 & \textbf{79.40}\\
        \bottomrule
    \end{tabular}
    \caption{Model performances on heuristically determined question types for RACE-Subset}
    \label{tab:heuristic_categories_perf}
\end{table}
%%%%%%%%%%%%%%%%%%%%%%%%%%%%%%%%%%%%%%%%%%%%%%%%%%%%%%%%%%%%%%%%%%%%%%%%%%%%%%%

%Category tables
\begin{table*}[!ht]
    \centering
    \begin{tabular}{p{3.5cm}|p{5.5cm}|p{5.5cm}}
        \toprule
        \textbf{Category} & \textbf{Description} & \textbf{Example}\\
        \bottomrule
        Linguistic Matching & Can be answered merely by matching words between the question and a sentence from the passage & \textbf{Passage Sentence:} Food cooks quickly in parabolic cookers \\ & & \textbf{Question:}If you want to cook food quickly, which kind of sun-cooker is your best choice?\\\hline
        Main Idea & Require topicality judgements & What's the best title for this passage?\\\hline
        Negation & Picking the wrong/incorrect statement & Which of the following statements is NOT true?\\\hline
        Dialogue & Can be inferred from a dialogue or direct speech in the passage & By saying "her pen dared travel where her eyes would not", the writer means\\\hline
        Math & Counting or mathematically combining facts & How many functions of snow are discussed in the passage?\\\hline
        Deductive & None of the above but can be answered precisely from the premise text & Which of the following statements is TRUE?\\\hline
        Inductive & None of the above and cannot be answered precisely from the text & How old is most likely the writer's father?\\
        \bottomrule
    \end{tabular}
    \caption{Reasoning Categories}
    \label{tab:reasoning_categories}
\end{table*}

\begin{table*}[!ht]
    \centering
    \begin{tabular}{p{0.25\textwidth}|p{0.65\textwidth}}
        \toprule
        \textbf{Type} & \textbf{Heuristics} \\
        \bottomrule
        Main Idea & Questions containing the words 'mainly', 'title', 'purpose' or 'topic'\\\hline
        Negation & Questions containing the 'not', 'except' or 'which of the following is wrong'\\\hline
        Dialogue & Passages containing more than 10 quotation marks (")\\\hline
        Math & Questions containing the words 'how many', 'how old' or 'how much'\\\hline
        Deductive & Questions containing the word 'true'\\\hline
        Fill in the Blanks (FITB) & Questions containing a blank (\_)\\
        \bottomrule
    \end{tabular}
    \caption{Heuristically Determined Question Types - RACE}
    \label{tab:heuristic_categories}
\end{table*}

\subsection{Multirc categories}
\label{app:analysis_multirc_categories}

\begin{table*}[!ht]
    \centering
    \begin{tabular}{@{}l|p{0.35\textwidth}|p{0.35\textwidth}@{}}
    \toprule
        \textbf{Type} & \textbf{Heuristic} & \textbf{Example}\\
    \toprule
        what (40\%) 
 & Starts With ['What', 'In what', 'With what', 'To what'] or Ends With [‘what?’]
 & What is the drawback of kinetic energy from hydro power? \\ \hline
        who (15\%) & Starts With ['Who', 'Whom', 'With whom', 'From whom', 'For whom'] or Ends With [‘who?’, ‘whom?’] & Who does Billy have the same color hair as?\\ \hline
        how (12\%)& Starts With [‘How’] & Approximately how much older is Charlie than Sylvia?\\ \hline
        why (10\%)& Starts With [‘Why’] & Why did Phoebe cry?\\ \hline
        assertion (5\%)& Starts With ['Could it', 'Will ', 'Was', 'Were', 'Has', 'Have', 'Does', 'Would', 'Did', 'Had', 'Is', 'Are', 'Do', 'Can', 'True or false'] & Was the Emperor hurt when the explosion damaged his carriage?\\ \hline
        which (5\%) & Starts With ['Which', 'In which'] & Which philosopher is said to have taught the young Confucius?\\ \hline
        double questions (4.5\%) & Contains ['and what', 'and how', 'and which', 'and where', 'and when', 'and why', 'and by whom', 'if not, what?'] or count("?") $>$ 1 & Where did money to fund the 9/11 plotters come from and where didn't it come from?\\ \hline
        when (3\%) & Starts With [‘When’]
 & When did the Romans set up a fortress at Aquae Sextiae (Aix-en-Provence)?\\ \hline
        where (3\%) & Starts With [‘Where’] or Ends With [‘where?’]
 & Where does the absorption part of digestion occur?\\
    \bottomrule
    \end{tabular}
    \caption{Heuristicaly Determined Question Types - MultiRC}
    \label{tab:heuritic_categories_multirc}
\end{table*}

\begin{table*}[!ht]
    \centering
    \begin{tabular}{p{0.6\textwidth}|l|p{0.2\textwidth}}
    \toprule
        \textbf{Example} & \textbf{Type} & \textbf{Remark}\\
    \toprule
        \textbf{Q:} What are two units of speed?
        & \multirow{2}{*}{what} & \multirow{2}{*}{Multiple answers}\\ 
        \textbf{A:} SI and MPH &&\\ \hline
        \textbf{Q:} What was the names and locations of two peers of bin Ladin?
        & \multirow{2}{*}{what} & Multiple answers,\\
        \textbf{A:} Blind Sheik - New Jersey &&Partially correct \\ \hline
        \textbf{Q:} What was Dennis Rodman's response when asked about his trip?
        & \multirow{2}{*}{what} & \multirow{2}{*}{Question in answer}\\
        \textbf{A:} When will we tire of this circus? &&\\ \hline
        \textbf{Q:} Who are the characters in this story?
        & \multirow{2}{*}{who} & \multirow{2}{*}{Multiple answers}\\
        \textbf{A:} David and Alannah && \\ \hline
        \textbf{Q:} Who are two members of Sarah's inner circle?
        & \multirow{2}{*}{who} & \multirow{2}{*}{Partially correct}\\ \textbf{A:} Ray &&\\ \hline
        \textbf{Q:} Explain the religious schism in both England and Scotland.
        & \multirow{2}{*}{uncategorized} & \multirow{2}{*}{Hard for Conversion} \\
        \textbf{A:} Scotland was protestant &&\\ \hline
        \textbf{Q:} What are the three ways in which Finnish reform can be seen?
        & \multirow{4}{*}{what} & Multiple answers, Partially correct\\
        \textbf{A:} The elevation of Finnish from a language of the common people to a national language equal to Swedish && \\
         
    \bottomrule
    \end{tabular}
    \caption{Example that are difficult for NLI under the constraints of the considered rules and neural model in the MultiRC dataset.}
    \label{tab:multirc_hard_examples}
\end{table*}
