# Supplementary material for: Looking Beyond Sentence-Level Natural Language Inference for Downstream Tasks
Source: arXiv:2009.09099 source file (2020-09-18)
Supplement: Supplementary file 3 [file hyperparams.tex]

\subsubsection{Evaluating Conversion Quality}
%\vspace{-100mm}
\begin{table}[!ht]
\centering
\resizebox{\columnwidth}{!}{%
\begin{tabular}{@{}l|c|c|c|c@{}}
\toprule
\textbf{Hyperparam} & \textbf{RACE} & \textbf{Dream} & \textbf{MultiRC} & \textbf{CosmosQA} \\ \midrule
learning rate       & 1e-5          & 1e-5           & 1e-5             & 1e-5              \\ \midrule
weight decay        & 0.01          & 0.01           & 0.01             & 0                 \\ \midrule
warmup steps        & 1300          & 400            & 160              & 80                \\ \midrule
batch size          & 16            & 32             & 32               & 24                \\ \midrule
max epochs          & 3             & 5              & 5                & 4                 \\ \bottomrule
\end{tabular}%
}
\caption{Hyperparam setting for the models trained on MCRC datasets (Q+A) from, that is for the results in the first column of Table \ref{tab:all-results}. \todo{Update this} }
\label{tab:hyperparams_q+a}
\end{table}

\subsubsection{Summary Correctness and semantic phenomena}
