# Supplementary material for: Looking Beyond Sentence-Level Natural Language Inference for Downstream Tasks
Source: arXiv:2009.09099 source file (2020-09-18)
Supplement: Supplementary file 4 [file premise_len.tex]

\comment{This seems very ad-hoc. Should we remove/put this in the Appendix?}
\label{subsec:qualitative_premise}

We noticed that the long passages in the question answering task resulted in an unnaturally long premise for the entailment task. Table \ref{tab:premise_len} lists the 90\textsuperscript{th} and 99\textsuperscript{th} percentile lengths of the passage for each of the datasets. We conjecture that intelligent selection of relevant sentences from the passage to effectively reduce the premise length for the entailment task would further improve performance. 

\begin{table}[h]
    \centering
    \begin{tabular}{c|c|c}
        \textbf{Dataset} & \textbf{90\textsuperscript{th} percentile} & \textbf{99\textsuperscript{th} percentile}\\
        \bottomrule
        RACE & 373 & 610 \\ \hline
        Dream & 251 & 575\\ \hline
        MultiRC & 397 & 470 \\ 
        \bottomrule
    \end{tabular}
    \caption{Passage lengths (based on tokens created using space) for the different datasets.}
    \label{tab:premise_len}
\end{table}
